# Supplementary material for: Rhythms of the collective brain: Metastable synchronization and cross-scale interactions in connected multitudes
Source: arXiv:1611.06831 ancillary file (2018-01-17)
Supplement: Supplementary file 1 [file supplementary.pdf]

# Supplementary Information

## Rhythms of the collective brain: Metastable synchronization and cross-scale interactions in connected multitudes

Miguel Aguilera

## S1 Data preprocessing

We use a data set of 1,444,051 tweets from 181,146 users, collected between 13 May 2011 and 31 May 2011. This data set was extracted from the Twitter streaming API, which provides information on the date and content of the tweet, as well as information about the sender, including location. Messages were captured when they contained one of the following hashtags or keywords (which were selected as some of the most relevant during the emergence of the 15M movement): #15M, 15-M, #democraciarealya, #tomalacalle, #Nolesvotes, #spanishrevolution, #acampadasol, #acampadabcn, #indignados, #notenemosmiedo, #nonosvamos, #yeswecamp. We filter messages in the data set using the location field in the description of the user that sent the message. Since the 15M was (at least during the first days) mainly an urban phenomena, we analyse geographical interactions between the 15 cities with more activity in Twitter during 17 days of the protests. We find the 15 names of cities most repeated in the data set, and counted messages corresponding to a specific city when the city name appeared in the location field. Since the location is a field of the description of the user, it does not necessarily correspond to the real location of the user at the moment the message was sent. We ran a test on geolocalized Twitter data from Spain, observing that for a set of 20.000 random tweets in a 80.25% the profile location corresponds with the actual geolocation of the user, giving the information of the user's location field a moderately high reliability.

## S2 Phase-locking statistics

Time series of activity at each city are generated by counting the number of messages from users located at the city in intervals of 60 seconds for a period comprising 17 days, starting at 2AM May 14th 2011. Each time series is filtered using Morlet wavelets at different frequencies. For each city $i$ and frequency $f$ we extract the phase content $\theta_x(f,t)$ for each moment of time $t$, with a frequency span between $[1.67 \cdot 10^{-3} Hz, 9.26 \cdot 10^{-5} Hz]$ (from 10 minutes to 3 hours) mapped into a logarithmic sequence with intervals of $10^{0.01}$.

Phase-locking values are defined for each pair of cities $i$ and $j$ as defined in Equation 1. We introduce a corrector factor $A_{ij}(t)$ to remove spurious synchronization when the network is inactive. $A_{ij}(t)$ is zero when the mean activity of node $i$ or node $j$ for a moving window of 30 minutes is below a threshold of 0.25 times its mean activation, which generally happened during some periods at night.

From phase-locking values we extract phase-locking links, which are activated when the phase-locking value is higher than 99% of a set of 200 surrogate time series we generate for purposes of statistical validation, as indicated in Equation 2. Surrogate time series are generated using amplitude adjusted Fourier transform using the TISEAN software (Available at http://www.mpipks-dresden.mpg.de/~tisean/Tisean_3.0.1/). Amplitude adjusted Fourier transform surrogates are time series that preserve the power spectrum of a distribution and a distribution of values, but remove the temporal correlations present in the original signal.

| Label | Frequency |
|---|---|
| $f_1$ | $1.52 \cdot 10^{-3} Hz$ |
| $f_2$ | $1.10 \cdot 10^{-3} Hz$ |
| $f_3$ | $6.78 \cdot 10^{-4} Hz$ |
| $f_4$ | $4.00 \cdot 10^{-4} Hz$ |
| $f_5$ | $2.90 \cdot 10^{-4} Hz$ |
| $f_6$ | $1.91 \cdot 10^{-4} Hz$ |
| $f_7$ | $1.29 \cdot 10^{-4} Hz$ |
| $f_8$ | $1.10 \cdot 10^{-4} Hz$ |

**Table S1. Frequencies of salient synchronization**. Table representing the frequency values corresponding to the peaks represented in Figure S1.B.

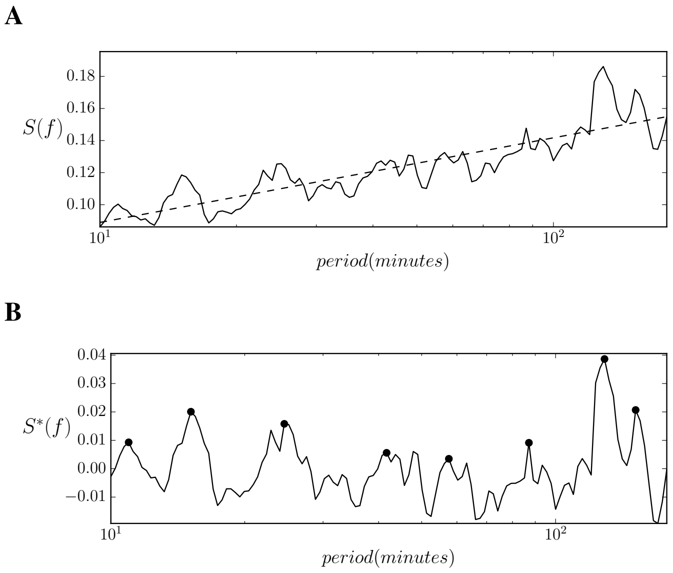


**Figure S1. Peaks of salient synchronization.** **(A)** Sum of total phase locking links $S(f)$ for each value of frequency (solid line). We detect a log-linear trend that we remove for detecting synchronization peaks. **(B)** Detrended $S(f)$ for each value of frequency (solid line). Synchronization peaks found using a two-dimensional wavelet transform (black dots).

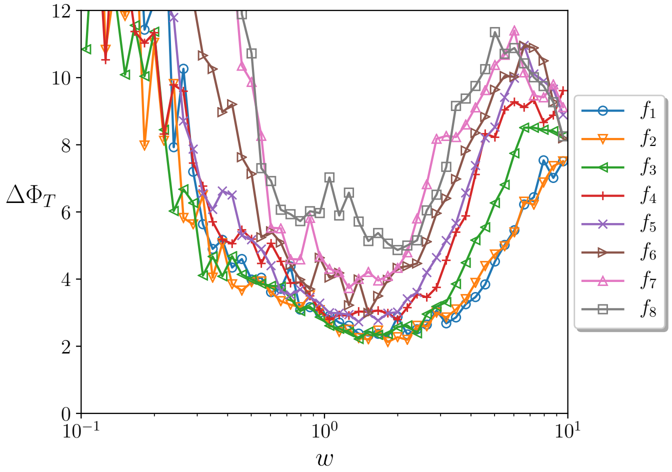


**Figure S2. Stability of synchronization patterns**. Average value of the sum of derivatives $\Delta\Phi_T(w)$ of the salient values of synchronization $\Delta\Phi_{ij}(t, f, w)$ for different multiplicators $w$ of the width of the wavelet windows. We find that small or large multiplicators reduce the stability of salient synchronization patterns, suggesting that wavelet filtering is a good strategy for defining the windows for phase-estimation filtering.

| Label | Number of transitions between states |
|---|---|
| $f_1$ | 2276 |
| $f_2$ | 1903 |
| $f_3$ | 1387 |
| $f_4$ | 922 |
| $f_5$ | 865 |
| $f_6$ | 692 |
| $f_7$ | 731 |
| $f_8$ | 641 |

**Table S2. Number of state transitions for each frequency**. Number of transitions between states $s$ from the data used for computing the Ising model at each selected frequency.

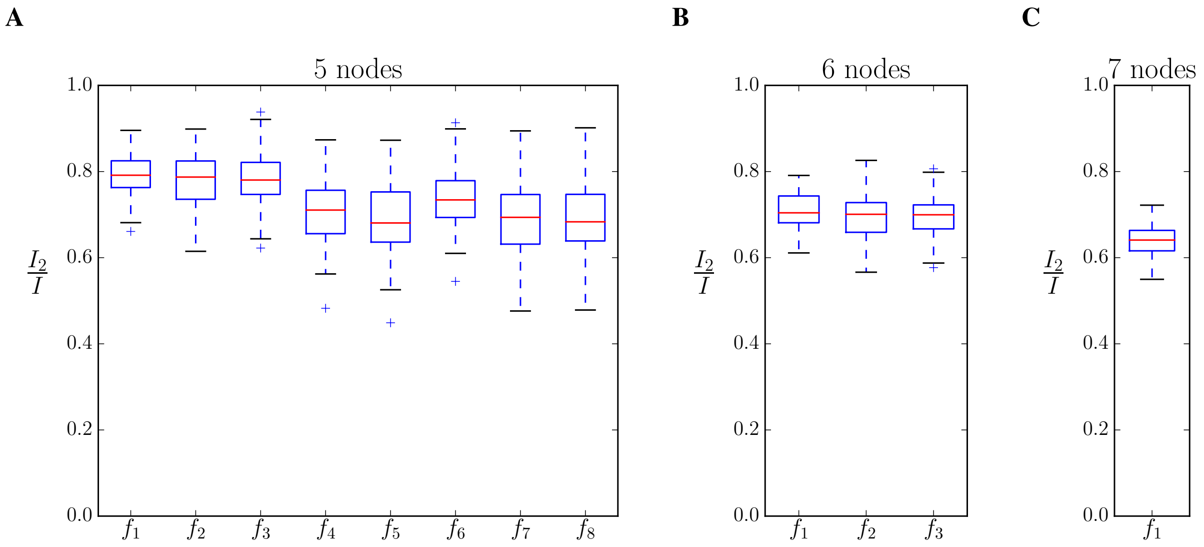


**Figure S3. Accuracy of the model**. Values of $\frac{I_2}{I}$ calculated for Ising models computed from subsets of combinations of nodes at at each frequency. Each boxplot represents the distribution of $\frac{I_2}{I}$ for 100 subsets of $n$ nodes at a specific frequency band selected randomly comparing the multi-information of the model and real data.

## S3 Detection of salient synchronization frequency bands

We localize frequency bands synchronization by detecting peaks of salient phase-locking links in the logarithmic frequency space. We compute the mean number of synchronization links for each frequency as the temporal mean of phase locking links at that frequency $S(f) = \langle \sum_{i,j} \Phi_{ij}(f,t) \rangle$ (Figure S1.A). As $S(f)$ increases with slower frequencies following approximately a log-linear trend, we approximate the trend computing a least squares first order polynomial fit respect to the logarithm of $f$ and remove it from $S(f)$ obtaining a detrended function. $S(f)^*$ In order to robustly detect peaks, we apply a two-dimensional wavelet transform of the detrended $S(f)$ over the vector of logarithmic frequencies. Using 10 Ricker wavelets of widths from 1 to 10 steps in the selected logarithmic range of frequency (i.e. a range of $[1.67 \cdot 10^{-3} Hz, 9.26 \cdot 10^{-5} Hz]$ logarithmically distributed with intervals of $10^{0.01}$) we compute the wavelet transform matrix and detect its ridge lines to find eight peaks of salient synchronization (code available at https://github.com/scipy/scipy/blob/v0.14.0/scipy/signal/_peak_finding.py#L410). As the position of the detected peaks vary slightly depending on the parameters employed, we adjust the position of each peaks by climbing to the nearest local maxima if one is found within a distance of two steps. In Figure S1.B we observe the result of the process and the 8 detected peaks. From these peaks we extract 8 frequencies $f_k$, with $k = 1, ..., 8$, indicating the position of the peaks in $S(f)$ (Table S1).

## S4 Validation of phase-detection and wavelet window length

As indicated in the manuscript, phase content $\theta_i(f,t)$ of the activity time series at city $i$ at time $t$ and frequency $f$ is extracted filtering the time series using Morlet wavelets, with a span of frequencies in the range $[1.67 \cdot 10^{-3}Hz,\ 9.26 \cdot 10^{-5}Hz]$ (from 10 minutes to 3 hours) logarithmically distributed with intervals of $10^{0.01}$. Morlet wavelets filter the signal using a Gaussian window. The width of the window is determined by the frequency of the wavelet oscillations, being the standard deviation of the Gaussian window equal to the period of the oscillations. The wavelet transform provides an arbitrary criterion for establishing the length of the filtering windows used for estimating the phase content of a signal (i.e. window length should be inversely proportional to the signal frequency). Other criteria could be using a fixed window length for all frequencies, as in the short-time Fourier transform. We explore which criteria is more appropriate for the data analyzed here. Since our analysis spans a wide range of frequencies, a wavelet transform appears as an appropriate choice. In this section we try to validate this intuition by comparing the results of different window lengths.

For doing so, we select the 8 synchronization frequencies selected in the previous section and analyze them using different window widths. For each frequency, we repeat the synchronization analysis from the section "Synchronization at multiple frequencies" of the manuscript multiplying the width of wavelet windows by a factor $w$.

For 51 values of $w$, logarithmically distributed between $[0.1, 10]$ we computed the values of $\phi_{ij}(f,t,w)$ for the time series and the 200 surrogate series, obtaining the values of salient synchronization $\Phi_{ij}(f,t,w)$ for each pair of nodes at specific times and frequencies. To evaluate the stability of the detected synchronization patters for each value of $w$, we compute the derivative of $\Phi_{ij}(f,t,w)$ respect to $w$ as $\Delta\Phi_{ij}(f,t,w) = \frac{1}{w}(\Phi_{ij}(f,t,w+dw) - \Phi_{ij}(f,t,w))/dw$, and the average of the sum of derivatives over the different pairs of cities as $\Delta\Phi_T(w) = \frac{1}{T}\sum_t \sum_{i,j} \Delta\Phi_{ij}(f,t,w)$, where $T$ is the total number of samples of the temporal series.

In Figure S2 we show $\Delta\Phi_T(w)$ for the 8 selected frequencies and the span of window widths. We find that most stable synchronization patterns are found around $w = 1$ for slower frequencies, and slightly larger values for faster frequencies (although those have a wider stability region. At extreme values of $w$ the patterns found become unstable. This suggests that, for our data, a wavelet transform is an adequate strategy to determine the phase contents of the signals, in comparison with other strategies as using fixed windows.

## S5 Number of samples required to compute probability distributions

When we compute multi-informations and transfer entropies from the data set, we face a compromise between the size of the probability distribution function of the system (corresponding to $2^N$ states) and the number of samples we employ for calculating it. In order to correctly compute these probability distributions, we need to ensure that the number of samples found in our data is sufficiently large for describing the frequency of occurrence of all possible states. Although the number of samples in our data is large, as data changes at different frequencies, slower frequencies may present a smaller number of transitions between states than fast frequencies, therefore offering a reduced effective sample of visited states.

In order to quantify the number of states visited at each frequency, we count the number of transitions between states $s$ used to infer the Ising models at each frequency (Table S2). Knowing that number, we can estimate a threshold of how many states can have a probability distribution to be accurately estimated from our samples at different frequencies. We arbitrarily establish a requirement of the number of transitions being larger than $2^4$ times the number of possible states of the objective probability distribution function. Although the exact value of the threshold is arbitrary, during the analysis we tried different thresholds to ensure the robustness of the results.

## S6 Multi-information measures for assessing the accuracy of maximum entropy models

Once we infer the maximum entropy models that correspond to the means and correlations found in phase-locking data, it is important to characterize what is the accuracy of the model, that is, to what extent the statistical model generated is mapping the data we used in the inference. The accuracy of the model can be further evaluated by asking how much of the correlative structure found in the data is captured. We can measure the overall strength of correlations in the network using multi-information, which is defined as the total reduction in entropy relative to an independent model $I = H[P_1] - H[P_r]$, where $H[P_r]$ is the entropy of the distribution of the real system whose data we are analysing and $H[P_1]$ is the entropy of an independent model. In our case, an independent model would be the equivalent of adjusting an Ising model in which the couplings are zero, and thus its energy function is defined as $E(s) = -\sum_i h_i s_i$. Multi-information can as well be used to compute the reduction of entropy of the distributions $P_2$ of the pairwise Ising model we inferred from data as $I_2 = H[P_1] - H[P_2]$. The ratio between these two quantities gives the fraction of the correlations captured by the pairwise Ising model:

$$\frac{I_2}{I} = \frac{H[P_1] - H[P_2]}{H[P_1] - H[P_r]} \tag{1}$$

Unfortunately, the data series available are not large enough for reliably computing $P_r$. The probability distribution $P_r$ has a number of possible states of $2^{15}$, while in our data the number of different states transited by the system is one or two orders of magnitude inferior, depending on the frequency. However, we can compute accurately subsets of the complete probability distribution $P_r(s')$, with $s' \subset s$. For each frequency, we count the number of transitions between states found in the time series in our data, and contrast that number with the dimension of the subset of the probability function using a number $n$ of nodes, i.e. $2^n$. We use an arbitrary threshold requiring the number of states being at least $2^4$ times larger than the number of values of the probability distribution function. Different thresholds yield slightly different results, although they don't change significantly the final results. We find that for frequencies from $f_4$ to $f_8$ we can compute reliably subsets with up to 5 nodes. For frequencies $f_2$ and $f_3$ the number increases to up to 6 and for $f_7$ it is 7 nodes.

In Figure S3 we can observe the distribution of the values of $\frac{I_2}{I}$ for 100 random choices of subsets for each number of nodes. For each subset of nodes, we fit a new Ising model mapping the distribution of the subset and compute its entropy to calculate $\frac{I_2}{I}$ We can observe that most of the subsets the values of $\frac{I_2}{I}$ indicate that between 60% and 80% of the correlations are captured (Table S3)

The limited availability of data, specially for slower frequencies, prevents us to compute the accuracy of the model for subsets with larger number of nodes. Future analysis applied to larger data sets should test if the accuracy of the model holds for capturing the correlations between larger subsets of nodes.

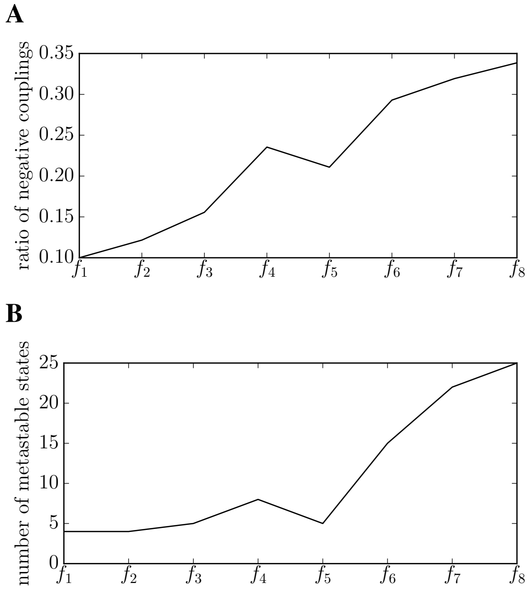


**Figure S4. Negative couplings and number of metastable states**. **(A)** Ratio of negative couplings for the inferred values of $J_{ij}$ for each frequency. **(B)** Count of the number of metastable states for each frequency.

## S7 Parameters of the Ising models

Here we display the parameters $h$ and $J$ inferred for the Ising models at each frequency. As we observe in Figure S6, as we move from faster to slower frequencies, the amplitude of $h$ and $J$ increases. As well, the percentage of negative couplings increases. We compute the ratio of negative couplings as:

$$r_{neg} = \frac{\sum_{i<j} |J_{ij}| - J_{ij}}{2 \sum_{i<j} |J_{ij}|} \tag{2}$$

In figure S4.A we can observe how the ratio of negative coupling increases with slower frequencies. It is known from spin glass theory that metastable states emerge when some of the couplings between variables are negative. In Figure S4 we can observe how there is a correlation between the ratio of negative couplings and the number of metastable states.

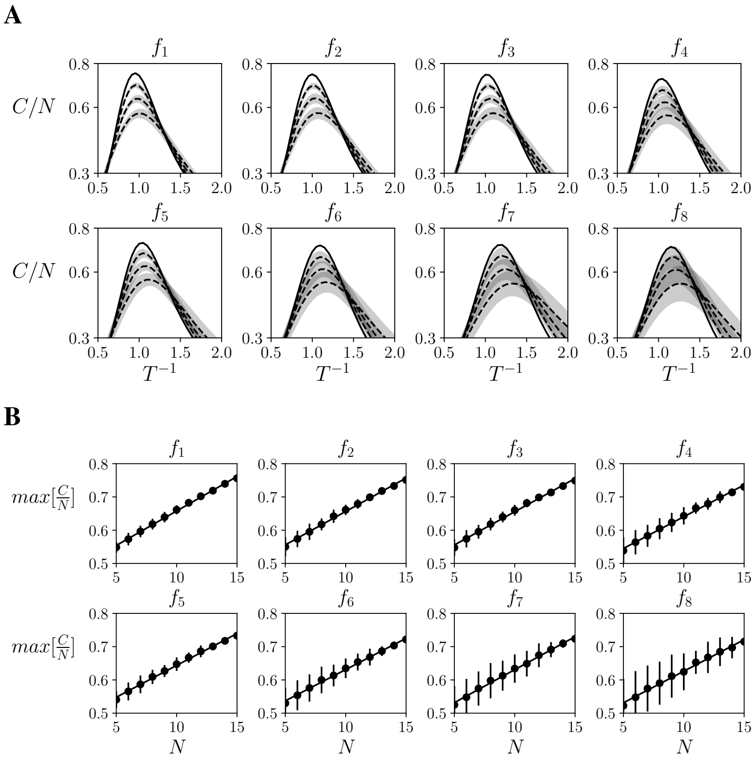


**Figure S5. Divergence of the heat capacity of the system**. **(A)** Normalized heat capacity $C(T)/N$ of the Ising models for sizes 6, 9, 12 (averaged over 100 random models) and 15, where the larger peaks corresponds to larger sizes. **(B)** Linear trend (solid line) of the peaks of $C(T)/N$ (dots) respect the size of the system.

## S8 Divergence of the heat capacity

At critical points, derivatives of thermodynamic quantities of the system as the entropy may diverge. An example of this is the heat capacity, whose divergence is a sufficient condition for criticality (though not a necessary one). To test the divergence of the heat capacity of the system, we extract Ising models of different sizes related to each frequency $f_k$. From sizes 5 to 15, we fit 100 Ising models inferring the set of means and correlation from $N$ random nodes of the system. For each size, we compute the normalized heat capacity $C(T)/N$ for the 100 models. In Figure S5.A we observe how the peaks of the heat capacity diverge for sizes $N = 6, 9, 12, 15$ (error bars are represented as a grey area). As size increases, the peak is higher and closer to $T = 1$. In Figure S5.B we represent the linear trend of the peaks from size 5 to 15. Trends are computed using a least squares first order polynomial fit. We identify trends with slopes in the range $[0.0188, 0.0207]$ and $R^2$ coefficients in the range $[0.993, 0.998]$. A linear trend of $max[C(T)/N]$ corresponds to a quadratic increment in the peak of the heat capacity $C(T)$ as $N$ increases, suggesting a divergence of the heat capacity of the system.

| Frequency | $n = 5$ | $n = 6$ | $n = 7$ |
|---|---|---|---|
| $f_1$ | $\mu = 0.790, \sigma = 0.0493$ | $\mu = 0.707, \sigma = 0.0434$ | $\mu = 0.696, \sigma = 0.0341$ |
| $f_2$ | $\mu = 0.778, \sigma = 0.0596$ | $\mu = 0.696, \sigma = 0.0520$ | |
| $f_3$ | $\mu = 0.782, \sigma = 0.0602$ | $\mu = 0.698, \sigma = 0.0497$ | |
| $f_4$ | $\mu = 0.707, \sigma = 0.0748$ | | |
| $f_5$ | $\mu = 0.692, \sigma = 0.0832$ | | |
| $f_6$ | $\mu = 0.739, \sigma = 0.0693$ | | |
| $f_7$ | $\mu = 0.685, \sigma = 0.0863$ | | |
| $f_8$ | $\mu = 0.687, \sigma = 0.0928$ | | |

**Table S3. Distributions of multi-information ratios**. Mean and standard deviation for each distribution in Figure S3.

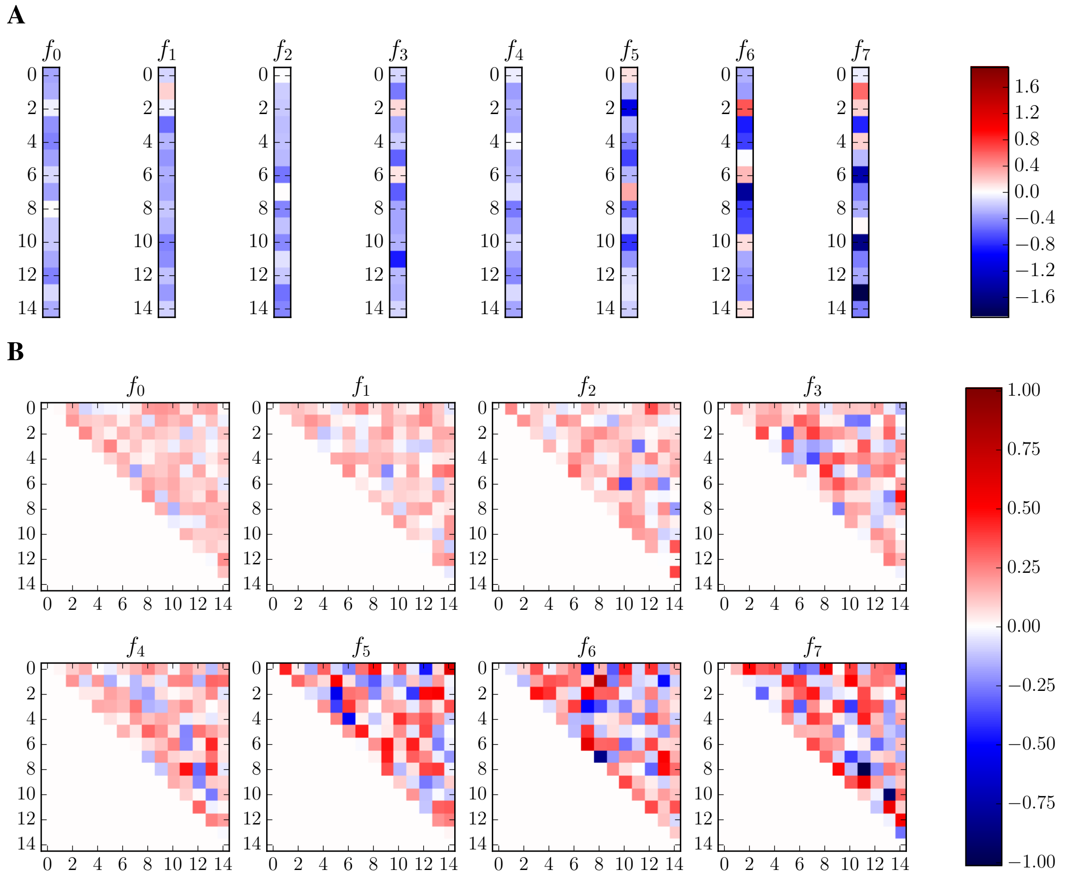

**Figure S6. Parameters of the Ising models**. For each frequency, we depict the parameters $h$ (**A**) and $J$ (**B**) of the inferred Ising models.

## S9 Metastable states

Metastable states are defined as states whose energy is lower than any of its adjacent states, where adjacency is defined by single spin flips. This means that in a deterministic state (i.e. a Hopfield network with $T = 0$) these points would act as attractors of the system. In our statistical model metastable states are points in which the system tends to be poised, since their probability is higher than any of its adjacent states. In table S4 we can observe a list of the metastable states for the model at each frequency. The probability of the metastable state $P(s)$ is just the probability of the corresponding state of the ising model, and the basin of attraction $B(s)$ is computed as the number of states (over a total of $2^1 5$) in the system that would fall in the mestastable state if the system operated with deterministic dynamics (i.e. $T = 0$).

## S10 Transfer entropy

Using the energy of the Ising models $E_{f_k}$ at different frequencies, we compute transfer entropy by discretizing energy functions into clusterized variables $E^*_{f_k}$. We apply natural Break classification through the Jenks-Caspall algorithm (code available at `https://github.com/domlysz/Jenks-Caspall.py`), which for each cluster minimizes the average deviation from the cluster's mean to determine the best arrangement of values intro different clusters. Since computing transfer entropies requires to compute joint probability functions with three variables, to meet the same criteria we used to compute multi-information, we use a number of 3 clusters to ensure that for all the frequencies we have a number of samples of transited states which is at least $2^4$ times larger than the values in the probability distribution. After discretizing the energy functions we compute the values of transfer entropies $\mathcal{T}_{kl}(\tau) = \mathcal{T}_{E^*_{f_k} \to E^*_{f_l}}(\tau)$ for values of $\tau$ in a range between $[1, 2^8]$ (i.e. from 1 minute to more than 4 hours) logarithmically distributed with intervals of $2^{0.25}$. Functions $\mathcal{T}_{kl}(\tau) = \mathcal{T}_{E^*_{f_k} \to E^*_{f_l}}(\tau)$ for different values of $k$ and $l$ are represented in Figure S7

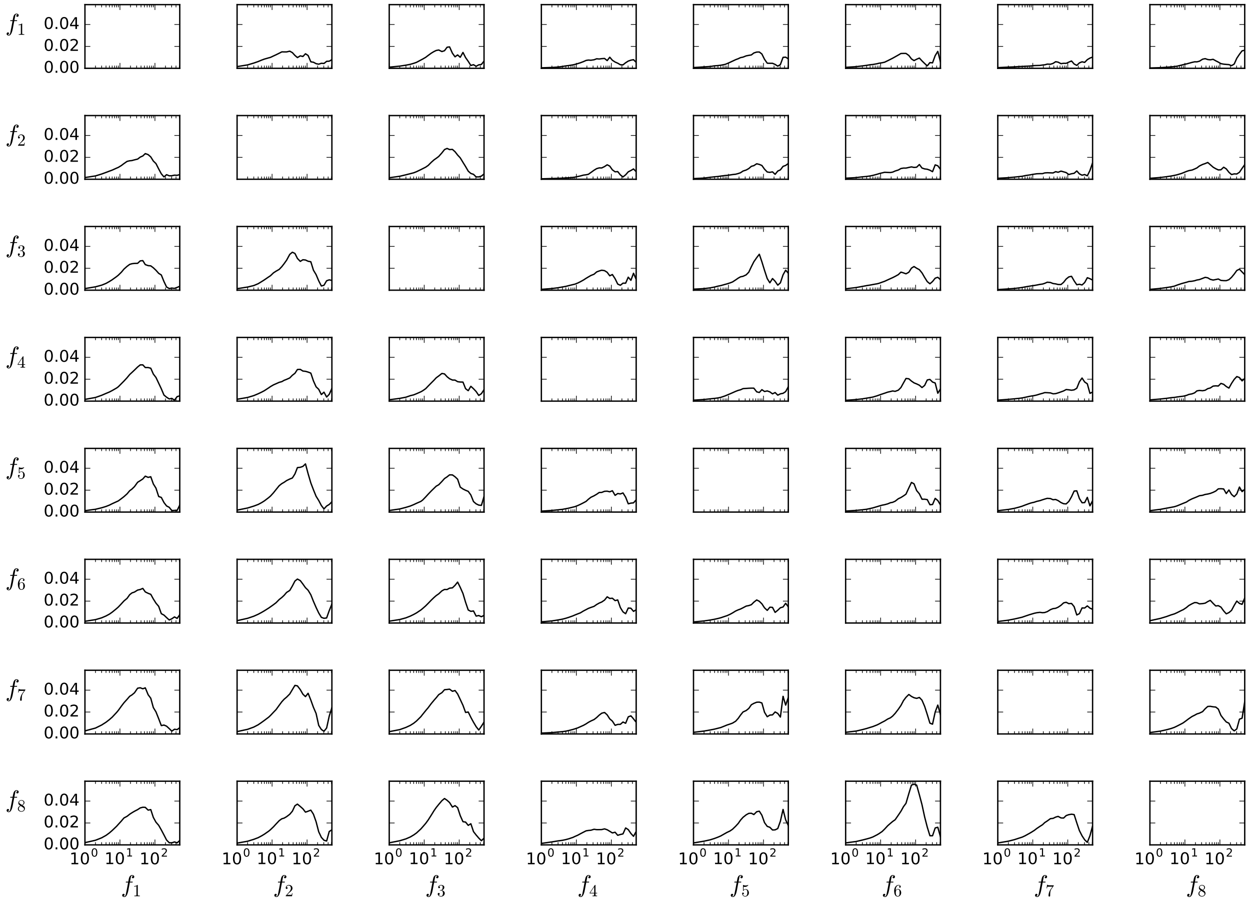


**Figure S7. Transfer entropy**. We represents functions $\mathscr{T}_{kl}(\tau) = \mathscr{T}_{E^*_{f_k} \to E^*_{f_l}}(\tau)$ for values of of $\tau$ in a range between $[1, 2^9]$ (i.e. from 1 minute to 8.5 hours) logarithmically distributed with intervals of $2^{0.25}$. Rows specify the value of $f_k$ while columns specify the value of $f_l$. For each graph, the vertical axis represents the value of transfer entropy and the horizontal axis the value of $\tau$ in minutes.

| Metastable state $s$ | $P(s)$ | $B(s)$ |
|---|---|---|
| $f_1$ | | |
| 000000000000000 | 0.333 | 28349 |
| 101000111110111 | $9.65 \cdot 10^{-6}$ | 139 |
| 101001101110111 | $7.97 \cdot 10^{-6}$ | 128 |
| 111111111111111 | $1.01 \cdot 10^{-4}$ | 4152 |
| $f_2$ | | |
| 000000000000000 | 0.283 | 29043 |
| 011011101001111 | $5.88E-06$ | 52 |
| 011111101111001 | $4.361E-06$ | 45 |
| 111111111111111 | $8.46E-05$ | 3628 |
| $f_3$ | | |
| 000000000000000 | 0.275 | 28934 |
| 100110010111111 | $1.48E-05$ | 102 |
| 111111110111101 | $4.46E-05$ | 883 |
| 111111111111100 | $5.64E-05$ | 1080 |
| 111111111111111 | $8.77E-05$ | 1769 |
| $f_4$ | | |
| 000000000000000 | 0.280 | 30379 |
| 001110101111001 | $1.27E-05$ | 47 |
| 101010111111111 | $1.84E-05$ | 97 |
| 101110000111110 | $4.94E-05$ | 292 |
| 111010110110111 | $3.98E-05$ | 1377 |
| 111010111110001 | $3.77E-05$ | 269 |
| 111101111010111 | $1.14E-05$ | 165 |
| 111110110111111 | $1.96E-05$ | 142 |
| $f_5$ | | |
| 000000000000000 | 0.256 | 29121 |
| 011011101110010 | $2.79 \cdot 10^{-5}$ | 246 |
| 110110010111001 | $4.43 \cdot 10^{-5}$ | 246 |
| 111111110110111 | $4.07 \cdot 10^{-5}$ | 849 |
| 111111111111111 | $8.91 \cdot 10^{-5}$ | 2306 |
| $f_6$ | | |
| 000000000000000 | 0.273 | 28445 |
| 000100101001111 | $6.17 \cdot 10^{-5}$ | 81 |
| 100000011100000 | $1.06 \cdot 10^{-3}$ | 485 |
| 100100111101001 | $4.44 \cdot 10^{-4}$ | 1268 |
| 100110010111001 | $7.67 \cdot 10^{-5}$ | 141 |
| 100110011001111 | $6.02 \cdot 10^{-5}$ | 228 |
| 100110011111011 | $6.20 \cdot 10^{-5}$ | 166 |
| 100111111111101 | $5.38 \cdot 10^{-5}$ | 125 |
| 101110111111111 | $2.64 \cdot 10^{-5}$ | 84 |
| 110001110101001 | $1.05 \cdot 10^{-4}$ | 257 |
| 110011011001111 | $7.23 \cdot 10^{-5}$ | 479 |
| 110111110111001 | $1.06 \cdot 10^{-4}$ | 232 |
| 110111111111111 | $4.31 \cdot 10^{-5}$ | 333 |
| 111100101100011 | $2.31 \cdot 10^{-5}$ | 39 |
| 111110000000111 | $1.37 \cdot 10^{-4}$ | 405 |

| Metastable state $s$ | $P(s)$ | $B(s)$ |
|---|---|---|
| $f_7$ | | |
| 000000000000000 | 0.194 | 23469 |
| 000000001111011 | $4.93 \cdot 10^{-4}$ | 466 |
| 000000010011011 | $7.83 \cdot 10^{-4}$ | 831 |
| 001000110111111 | $1.95 \cdot 10^{-4}$ | 642 |
| 001001010111001 | $2.90 \cdot 10^{-4}$ | 301 |
| 001010101100110 | $2.56 \cdot 10^{-5}$ | 35 |
| 001011010111111 | $7.29 \cdot 10^{-5}$ | 151 |
| 010000111011011 | $1.39 \cdot 10^{-5}$ | 66 |
| 011001111111001 | $2.68 \cdot 10^{-5}$ | 111 |
| 011010001110000 | $2.92 \cdot 10^{-4}$ | 304 |
| 011011110110100 | $1.59 \cdot 10^{-5}$ | 41 |
| 011011111110011 | $1.70 \cdot 10^{-5}$ | 71 |
| 011011111111111 | $2.63 \cdot 10^{-5}$ | 180 |
| 101000101111111 | $1.24 \cdot 10^{-4}$ | 800 |
| 101001110111101 | $8.42 \cdot 10^{-5}$ | 236 |
| 101100100000100 | $1.56 \cdot 10^{-3}$ | 990 |
| 111010101110100 | $1.71 \cdot 10^{-4}$ | 193 |
| 111011001010000 | $3.53 \cdot 10^{-4}$ | 934 |
| 111011110010100 | $2.87 \cdot 10^{-5}$ | 119 |
| 111101101000001 | $8.77 \cdot 10^{-4}$ | 1425 |
| 111111100000100 | $4.11 \cdot 10^{-4}$ | 401 |
| 111111101110101 | $2.17 \cdot 10^{-4}$ | 1002 |
| $f_8$ | | |
| 000000000000000 | 0.241 | 19686 |
| 000110000101101 | $6.14 \cdot 10^{-4}$ | 340 |
| 000110011100101 | $1.52 \cdot 10^{-4}$ | 160 |
| 001110010101101 | $1.94 \cdot 10^{-4}$ | 213 |
| 001111010001101 | $1.02 \cdot 10^{-4}$ | 84 |
| 010000000111000 | $1.14 \cdot 10^{-3}$ | 716 |
| 010000000111101 | $5.60 \cdot 10^{-4}$ | 836 |
| 010111000111101 | $3.07 \cdot 10^{-4}$ | 281 |
| 011000100111001 | $3.86 \cdot 10^{-4}$ | 399 |
| 011001110000000 | $6.08 \cdot 10^{-4}$ | 463 |
| 011111010101101 | $1.27 \cdot 10^{-4}$ | 286 |
| 100111011000000 | $9.33 \cdot 10^{-4}$ | 2250 |
| 101010011000000 | $2.86 \cdot 10^{-3}$ | 2021 |
| 101110000101101 | $2.27 \cdot 10^{-4}$ | 247 |
| 101110011100101 | $2.54 \cdot 10^{-4}$ | 263 |
| 110010001110101 | $2.63 \cdot 10^{-4}$ | 764 |
| 110100000101110 | $8.45 \cdot 10^{-5}$ | 156 |
| 110111000111100 | $3.54 \cdot 10^{-4}$ | 591 |
| 110111001110101 | $3.26 \cdot 10^{-4}$ | 263 |
| 111000000010101 | $3.57 \cdot 10^{-4}$ | 128 |
| 111010000111101 | $1.06 \cdot 10^{-3}$ | 798 |
| 111011111000000 | $5.09 \cdot 10^{-4}$ | 860 |
| 111011111110101 | $8.33 \cdot 10^{-5}$ | 144 |
| 111111000111101 | $8.14 \cdot 10^{-4}$ | 614 |
| 111111011101110 | $7.86 \cdot 10^{-5}$ | 205 |

**Table S4. Metastable states**. Metastable state $s$ (where positive spins are marked with 1$s$ and negative with 0$s$), probability of the metastable state $P(s)$ and basin of attraction of the metastable state $B(s)$.
